# Supplementary material for: Summarizing Community-based Question-Answer Pairs
Source: arXiv:2211.09892 source file (2022-11-17)
Supplement: Supplementary file 1 [file appendix.tex]

\section{The \corpus Corpus}
% \todo{Detailed information about product categories etc.}
\tingyao{do we still need this?} \xiaolan{I think we can remove this.}

\section{Annotation Interface}
\label{sec:appendix:post-edit}
\Cref{fig:rewrite} shows the interface of QA post-edit task for crowd workers. In the instruction, we provide product link and QA examples referred to our annotation rules. We also put the rules on the right side of each question to help workers recall when they post-edit. We set up warning signs to remind workers for errors but they can still submit if they think it is reasonable.

\begin{figure*}
    \centering
    \includegraphics[width=0.8\textwidth]{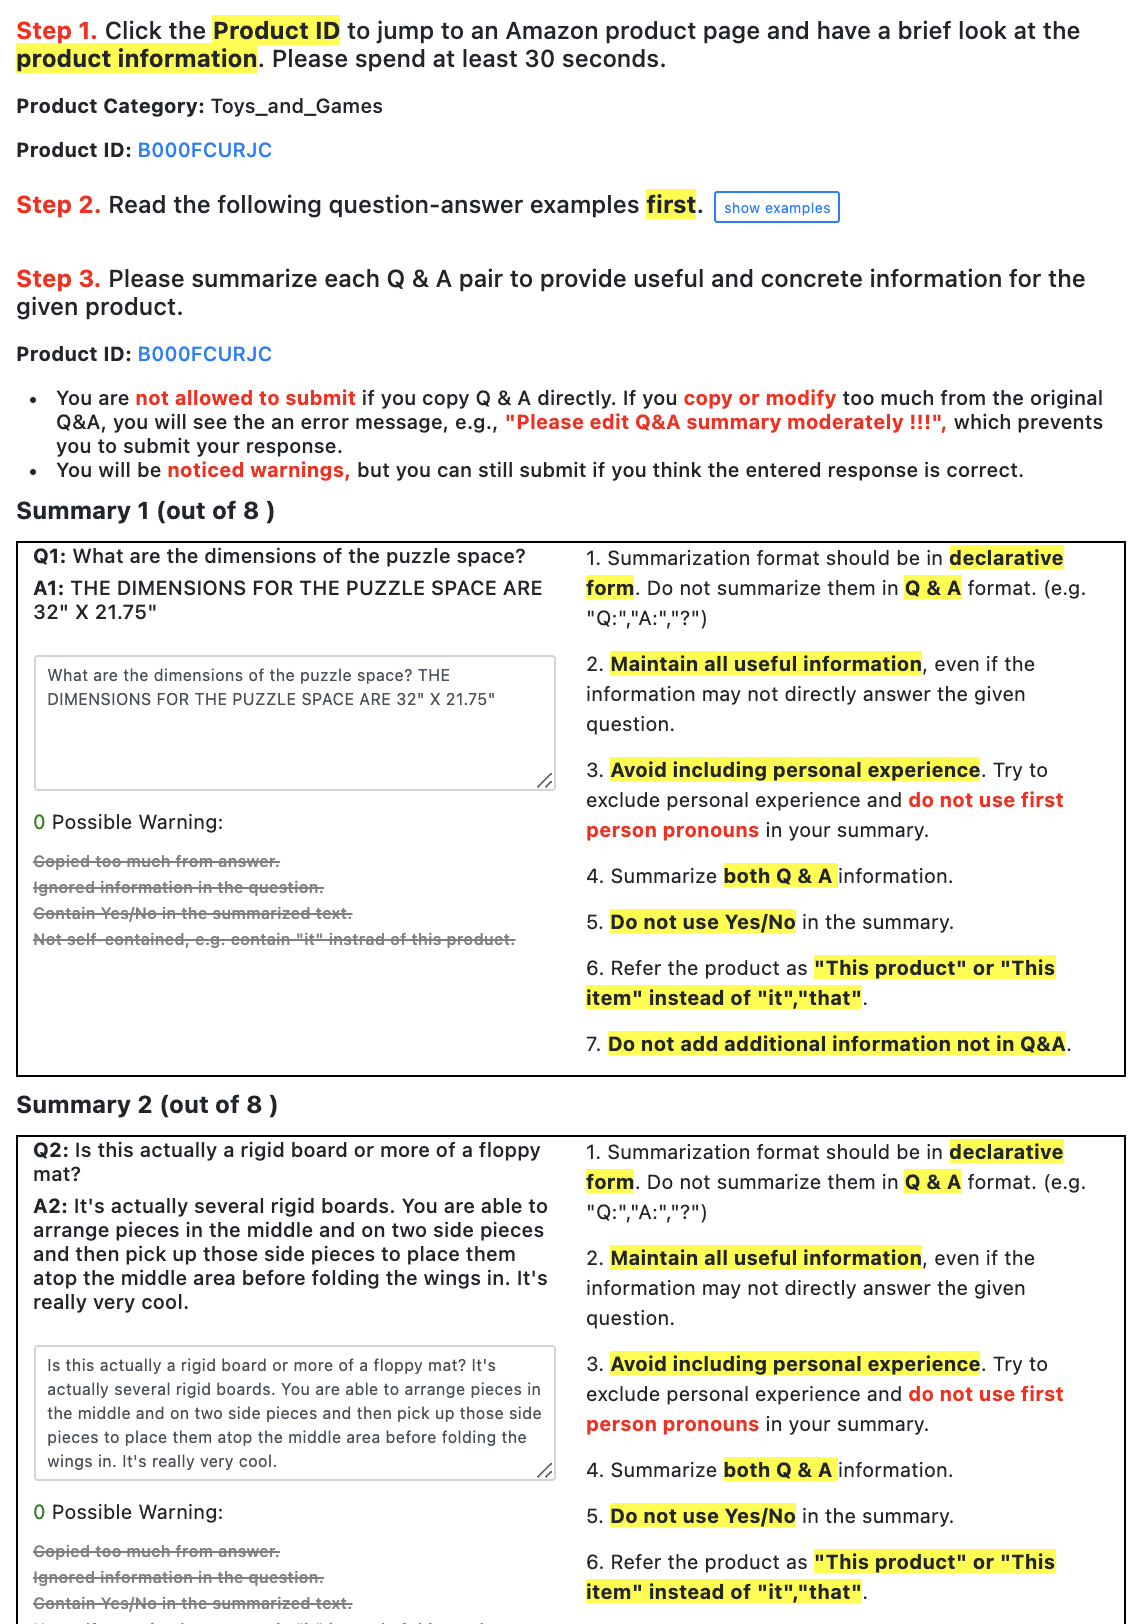}
    \caption{Interface of the QA post-edit annotation task. To assist annotators, we provided the product link for reference and use multiple rules to control the quality of the annotation. }
    \label{fig:rewrite}
\end{figure*}

\section{Model details}
\label{sec:appendix:model-details}

% \section{Example Appendix}
% \label{sec:appendix}
